# Supplementary material for: PAC-Bayesian Learning of Aggregated Binary Activated Neural Networks with Probabilities over Representations
Source: arXiv:2110.15137 source file (2023-04-14)
Supplement: Supplementary file 1 [file appendix_algorithms.tex]

We provide a detailed view on the forward propagation algorithms of ABNet and its stochastic counterpart, presented in Section~\ref{section:dynamic_programming}. We use $R' \sim \Ucal_{n}(R)$ to denote that $R'$ consists of $n$ draws (with replacement) from a uniform distribution on $R$. 

\begin{algorithm}[H]
 	\caption{ABNet}
	\tt\small
 		\begin{algorithmic}[1]
 		    \Require{$\xbf \in \Rbb^{d_0}$ and $\Bcal_M = \langle \Wbf_k \rangle_{k=1}^{L}$, with $\Wbf_k \in \Rbb^{d_{k-1} \times d_k} \; \forall 1 \leq k \leq L$}
 		    \vspace{2mm}
 			\State{$\Pbf \leftarrow \bigg[\prod_{i=1}^{d_1}  \bigg(\frac{1}{2} + \frac{\sbf_1^i}{2} \Erf\big(\frac{\Wbf_{1}^i \cdot \xbf}{\sqrt{2} \lVert \xbf \rVert}\big)\bigg)\bigg]_{\sbf_1 \in R_1}$ }
 			\For{$k \in \{2, \dots, L\}$}
 			    \State{$\Psibf = \bigg[\prod_{i=1}^{d_k} \bigg(\frac{1}{2} + \frac{\mathbf{s}_k^i}{2} \Erf\big(\frac{\mathbf{W}_{k}^i \cdot \mathbf{s}_{k-1}}{\sqrt{2 d_{k-1}}}\big)\bigg)\bigg]_{\mathbf{s}_{k} \in R_{k},\mathbf{s}_{k-1} \in R_{k-1}}$}
 				\State{$\mathbf{P} \leftarrow \mathbf{\Psi} \cdot \mathbf{P}$ }
 			\EndFor
 			\vspace{2mm}
 		\State{\Return{$\begin{bmatrix}1, -1\end{bmatrix} \cdot \mathbf{P}$}}
 	\end{algorithmic}
 	\label{algo:abNet}
 \end{algorithm}

\begin{algorithm}[H]
 	\caption{Stochastic ABNet}
	\tt\small
 		\begin{algorithmic}[1]
 		    \Require{$\xbf \in \Rbb^{d_0}$, $n \in \Nbb$ and $\Bcal_M = \langle \Wbf_k \rangle_{k=1}^{L}$, with $\Wbf_k \in \Rbb^{d_{k-1} \times d_k} \; \forall 1 \leq k \leq L$}
 		    \vspace{2mm}
 		    \State{$R'_1 \sim \Ucal_{n}(R_1)$}
 			\State{$\Pbf \leftarrow \bigg[\prod_{i=1}^{d_1}  \bigg(\frac{1}{2} + \frac{\sbf_1^i}{2} \Erf\big(\frac{\Wbf_{1}^i \cdot \xbf}{\sqrt{2} \lVert \xbf \rVert}\big)\bigg)\bigg]_{\sbf_1 \in R'_1}$ }
 			\State{$\Pbf \leftarrow \frac{\Pbf}{\sum_{\sbf_1 \in R'_1} \Pbf[\sbf_1]}$}
 			\For{$k \in \{2, \dots, L\}$}
 			\vspace{2mm}
 			    \State{$R'_k \sim \Ucal_{n}(R_k)$}
 			    \State{$\Psibf = \bigg[\prod_{i=1}^{d_k} \bigg(\frac{1}{2} + \frac{\mathbf{s}_k^i}{2} \Erf\big(\frac{\mathbf{W}_{k}^i \cdot \mathbf{s}_{k-1}}{\sqrt{2 d_{k-1}}}\big)\bigg)\bigg]_{\mathbf{s}_{k} \in R'_{k},\mathbf{s}_{k-1} \in R'_{k-1}}$}
 				\State{$\mathbf{P} \leftarrow \mathbf{\Psi} \cdot \mathbf{P}$ }
 				\State{$\Pbf \leftarrow \frac{\Pbf}{\sum_{\sbf_k \in R'_k} \Pbf[\sbf_k]}$}
 			\EndFor
 			\vspace{2mm}
 		\State{\Return{$\sum_{\sbf_L \in R'_L} \sbf_L \Pbf[\sbf_L]$}}
 	\end{algorithmic}
 	\label{algo:stochastic_abNet}
 \end{algorithm}
