# Supplementary material for: PAC-Bayesian Learning of Aggregated Binary Activated Neural Networks with Probabilities over Representations
Source: arXiv:2110.15137 source file (2023-04-14)
Supplement: Supplementary file 2 [file appendix_experiments.tex]

\begin{table}[ht]
    \centering
    \caption{Extended experiment results with standard deviation on wide architectures (with PBGNet and ABNet \textit{stochastic} versions) over the 5 repetitions for selected models: number of hidden layers ($L{-}1$), width (d), bound value and error rate on the train data (Error$_{S}$)  and on the test data for the model (Error$_{T}$) and the associated \emph{Maximum-A-Posteriori} BAM (MAP). 
    }
    \label{tab:selected_models_overview_mat_wide}
    \setlength{\tabcolsep}{5pt}
    {\small
    \begin{tabular}{llcccccc}
    \toprule
    Dataset & Model & $L{-}1$ &  $d$ & Bound & Error$_{S}$ & Error$_{T}$ & MAP\\
    \midrule
    \multirow{7}{*}{ads} 
    & PBGNet &  3 & 10 & 0.213 $\pm$ 0.004 & 0.140 $\pm$ 0.003 & 0.141 $\pm$ 0.010 & 0.141 $\pm$ 0.010 \\
    & ABNet &  2 & 10 & 0.216 $\pm$ 0.004 & 0.140 $\pm$ 0.003 & 0.141 $\pm$ 0.010 & 0.141 $\pm$ 0.010 \\
    & PBGNet$_{\ell}$ &  3 & 10 & 1.000 $\pm$ 0.000 & 0.020 $\pm$ 0.003 & 0.026 $\pm$ 0.006 & 0.028 $\pm$ 0.003 \\
    & ABNet$_{\ell}$ &  2 & 50 & 1.000 $\pm$ 0.000 & 0.020 $\pm$ 0.005 & 0.026 $\pm$ 0.005 & 0.025 $\pm$ 0.004 \\
    & EBP &  3 & 10 & -- & 0.005 $\pm$ 0.002 & 0.035 $\pm$ 0.006  & 0.049 $\pm$ 0.008  \\
    & BC & 1 & 10 & -- & 0.021 $\pm$ 0.005 & 0.032 $\pm$ 0.005 & \textcolor{lightgray}{0.032 $\pm$ 0.005} \\
    & BNN &  1 & 100 & -- & 0.029 $\pm$ 0.004 & 0.032 $\pm$ 0.005 & \textcolor{lightgray}{0.032 $\pm$ 0.005} \\
    \midrule
    \multirow{7}{*}{adult} 
    & PBGNet &  1 & 10 & 0.216 $\pm$ 0.001 & 0.156 $\pm$ 0.001 & 0.159 $\pm$ 0.002 & 0.158 $\pm$ 0.002 \\
    & ABNet &  1 & 10 & 0.216 $\pm$ 0.000 & 0.156 $\pm$ 0.001 & 0.160 $\pm$ 0.002 & 0.158 $\pm$ 0.002 \\ 
    & PBGNet$_{\ell}$ &  2 & 10 & 0.360 $\pm$ 0.004 & 0.146 $\pm$ 0.001 & 0.151 $\pm$ 0.002 & 0.164 $\pm$ 0.000  \\
    & ABNet$_{\ell}$ &  3 & 10 & 0.541 $\pm$ 0.033 & 0.143 $\pm$ 0.001 & 0.151 $\pm$ 0.002 & 0.151 $\pm$ 0.002 \\
    & EBP   & 2 & 100 & -- & 0.049 $\pm$ 0.002 & 0.186 $\pm$ 0.001  & 0.189 $\pm$ 0.003  \\
    & BC    & 1 & 50 & -- & 0.160 $\pm$ 0.003 & 0.164 $\pm$ 0.001 & \textcolor{lightgray}{0.164 $\pm$ 0.001} \\
    & BNN   & 1 & 100 & -- & 0.157 $\pm$ 0.002 & 0.165 $\pm$ 0.002 & \textcolor{lightgray}{0.165 $\pm$ 0.002} \\
    \midrule
    \multirow{7}{*}{mnist17} 
    & PBGNet &  1 & 10 & 0.041 $\pm$ 0.000 & 0.005 $\pm$ 0.000 & 0.006 $\pm$ 0.001 & 0.006 $\pm$ 0.001  \\
    & ABNet &  1 & 10 & 0.041 $\pm$ 0.000 & 0.005 $\pm$ 0.000 & 0.006 $\pm$ 0.001 & 0.006 $\pm$ 0.001 \\
    & PBGNet$_{\ell}$ &  2 & 10 & 1.000 $\pm$ 0.000 & 0.002 $\pm$ 0.001 & 0.005 $\pm$ 0.001 & 0.006 $\pm$ 0.001\\
    & ABNet$_{\ell}$ &  3 & 10 & 0.607 $\pm$ 0.084 & 0.002 $\pm$ 0.000 & 0.005 $\pm$ 0.001 & 0.005 $\pm$ 0.001 \\
    & EBP & 2 & 10 & -- & 0.000 $\pm$ 0.000 & 0.005 $\pm$ 0.000 & 0.005 $\pm$ 0.001  \\
    & BC & 3 & 50 & -- & 0.003 $\pm$ 0.001 & 0.006 $\pm$ 0.001 & \textcolor{lightgray}{0.006 $\pm$ 0.001} \\
    & BNN & 1 & 100 & -- & 0.004 $\pm$ 0.001 & 0.007 $\pm$ 0.001 & \textcolor{lightgray}{0.007 $\pm$ 0.001} \\
    \midrule
    \multirow{7}{*}{mnist49} 
    & PBGNet &  1 & 10 & 0.149 $\pm$ 0.007 & 0.037 $\pm$ 0.001 & 0.037 $\pm$ 0.004 & 0.036 $\pm$ 0.004  \\
    & ABNet &  1 & 10 & 0.147 $\pm$ 0.007 & 0.038 $\pm$ 0.001 & 0.037 $\pm$ 0.004 & 0.036 $\pm$ 0.004 \\
    &  PBGNet$_{\ell}$ &  1 & 50 & 0.992 $\pm$ 0.001 & 0.004 $\pm$ 0.000 & 0.012 $\pm$ 0.003 & 0.012 $\pm$ 0.003 \\
    & ABNet$_{\ell}$ &  3 & 10 & 1.000 $\pm$ 0.000 & 0.024 $\pm$ 0.001 & 0.029 $\pm$ 0.003 & 0.027 $\pm$ 0.003 \\
    & EBP   & 2 & 10 & -- & 0.001 $\pm$ 0.001 & 0.021 $\pm$ 0.004 & 0.026 $\pm$ 0.004 \\
    & BC    & 1 & 100 & -- & 0.005 $\pm$ 0.001 & 0.015 $\pm$ 0.003 & \textcolor{lightgray}{0.015 $\pm$ 0.003}\\
    & BNN   & 1 & 100 & -- & 0.011 $\pm$ 0.002 & 0.023 $\pm$ 0.003 & \textcolor{lightgray}{0.023 $\pm$ 0.003} \\
    \midrule
    \multirow{7}{*}{mnist56} 
    %& PBGNet &  1 & 10 & 0.089 & 0.021 & 0.029 & 0.030  \\
    & PBGNet &  1 & 10 & 0.090 $\pm$ 0.001 & 0.023 $\pm$ 0.001 & 0.025 $\pm$ 0.003 & 0.024 $\pm$ 0.003 \\ 
    %& ABNet &  1 & 10 & 0.089 & 0.021 & 0.029 & 0.029 \\
    & ABNet  & 1 & 10 & 0.090 $\pm$ 0.001 & 0.023 $\pm$ 0.001 & 0.025 $\pm$ 0.003 & 0.024 $\pm$ 0.003 \\ 
    %& PBGNet$_{\ell}$ &  1 & 50 & 0.989 & 0.002 & 0.011 & 0.012  \\
    & PBGNet$_{\ell}$ &  1 & 50 & 0.974 $\pm$ 0.017 & 0.003 $\pm$ 0.001 & 0.008 $\pm$ 0.002 & 0.008 $\pm$ 0.003 \\ 
    %& ABNet$_{\ell}$ & 1 & 10 & 1.000 & 0.007 & 0.018 & 0.018 \\
    & ABNet$_{\ell}$  & 1 & 10 & 1.000 $\pm$ 0.000 & 0.010 $\pm$ 0.002 & 0.017 $\pm$ 0.002 & 0.016 $\pm$ 0.002 \\ 
    & EBP   & 2 & 10 & -- & 0.000 $\pm$ 0.000 & 0.019 $\pm$ 0.004 & 0.021 $\pm$ 0.005 \\
    & BC & 3 & 50 & -- & 0.004 $\pm$ 0.001 & 0.010 $\pm$ 0.003 & \textcolor{lightgray}{0.010 $\pm$ 0.003} \\
    & BNN & 1 & 100 & -- & 0.004 $\pm$ 0.002 & 0.012 $\pm$ 0.001 & \textcolor{lightgray}{0.012 $\pm$ 0.001} \\
    \midrule
    \multirow{7}{*}{mnistLH} 
    & PBGNet &  1 & 10 & 0.167 $\pm$ 0.010 & 0.058 $\pm$ 0.013 & 0.059 $\pm$ 0.010 & 0.060 $\pm$ 0.010 \\
    & ABNet &  2 & 10 & 0.187 $\pm$ 0.003 & 0.087 $\pm$ 0.007 & 0.088 $\pm$ 0.006 & 0.087 $\pm$ 0.005  \\
    &  PBGNet$_{\ell}$ &  1 & 100 & 0.998 $\pm$ 0.001 & 0.006 $\pm$ 0.001 & 0.022 $\pm$ 0.001 & 0.024 $\pm$ 0.002 \\
    & ABNet$_{\ell}$ &  3 & 10 & 0.895 $\pm$ 0.021 & 0.050 $\pm$ 0.005 & 0.060 $\pm$ 0.005 & 0.058 $\pm$ 0.006  \\
    & EBP   & 1 & 100 & -- & 0.001 $\pm$ 0.000 & 0.027 $\pm$ 0.001  & 0.032 $\pm$ 0.002  \\
    & BC    & 1 & 100 & -- & 0.013 $\pm$ 0.002 & 0.027 $\pm$ 0.001 & \textcolor{lightgray}{0.027 $\pm$ 0.001} \\
    & BNN   & 1 & 100 & -- & 0.023 $\pm$ 0.001 & 0.036 $\pm$ 0.001 & \textcolor{lightgray}{0.036 $\pm$ 0.001} \\
    \midrule
    \multirow{5}{*}{CIFAR10 - Truck / Car} 
    & PBGNet & 1 & 10 & 0.376 $\pm$ 0.001 & 0.234 $\pm$ 0.003 & 0.237 $\pm$ 0.002 & 0.233 $\pm$ 0.003 \\
    & ABNet & 1 & 10 & 0.375 $\pm$ 0.001 & 0.235 $\pm$ 0.001 & 0.239 $\pm$ 0.003 & 0.234 $\pm$ 0.002 \\ 
    & PBGNet$_{\ell}$ & 1 & 50 & 0.998 $\pm$ 0.001 & 0.161 $\pm$ 0.009 & 0.197 $\pm$ 0.006 & 0.197 $\pm$ 0.004 \\
    & ABNet$_{\ell}$ & 2 & 50 & 0.794 $\pm$ 0.030 & 0.216 $\pm$ 0.004 & 0.226 $\pm$ 0.002 & 0.225 $\pm$ 0.002 \\
    & EBP & 2 & 50 & -- & 0.005 $\pm$ 0.002 & 0.184 $\pm$ 0.008 & 0.227 $\pm$ 0.015  \\
    \midrule
    \multirow{5}{*}{CIFAR10 - Cat / Dog} 
    & PBGNet &  1 & 10 & 0.501 $\pm$ 0.000 & 0.418 $\pm$ 0.001 & 0.418 $\pm$ 0.005 & 0.417 $\pm$ 0.001 \\
    & ABNet & 1 & 10 & 0.500 $\pm$ 0.001 & 0.418 $\pm$ 0.001 & 0.423 $\pm$ 0.006 & 0.418 $\pm$ 0.001 \\
    & PBGNet$_{\ell}$ & 2 & 100 & 1.000 $\pm$ 0.000 & 0.380 $\pm$ 0.015 & 0.398 $\pm$ 0.005 & 0.399 $\pm$ 0.005 \\
    & ABNet$_{\ell}$ & 1 & 10 & 0.708 $\pm$ 0.051 & 0.390 $\pm$ 0.011 & 0.402 $\pm$ 0.005 & 0.400 $\pm$ 0.006 \\
    & EBP & 2 & 50 & -- & 0.012 $\pm$ 0.007 & 0.183 $\pm$ 0.008 & 0.226 $\pm$ 0.012 \\
    \midrule
    \multirow{5}{*}{CIFAR10 - Bird / Plane} 
    & PBGNet & 1 & 10 & 0.440 $\pm$ 0.000 & 0.338 $\pm$ 0.001 & 0.336 $\pm$ 0.003 & 0.331 $\pm$ 0.001 \\
    & ABNet & 1 & 10 & 0.439 $\pm$ 0.000 & 0.340 $\pm$ 0.001 & 0.334 $\pm$ 0.005 & 0.332 $\pm$ 0.001 \\
    & PBGNet$_{\ell}$ & 1 & 100 & 1.000 $\pm$ 0.000 & 0.192 $\pm$ 0.020 & 0.262 $\pm$ 0.005 & 0.262 $\pm$ 0.002 \\
    & ABNet$_{\ell}$ & 3 & 10 & 0.764 $\pm$ 0.028 & 0.283 $\pm$ 0.005 & 0.293 $\pm$ 0.005 & 0.295 $\pm$ 0.003 \\
    & EBP & 2 & 50 & -- & 0.007 $\pm$ 0.005 & 0.183 $\pm$ 0.010 & 0.232 $\pm$ 0.015  \\
    \bottomrule
    \end{tabular}
    }
\end{table}

\begin{table}[ht]
    \centering
    \caption{Extended experiments: number of hidden layers ($L{-}1$), width (d), both C and KL divergence values from the computation of the corresponding bound, learning rate (LR) and epoch providing the best model (Best epoch) given the algorithm stops after 100 epochs. Made on three binary variants of the CIFAR10 \cite{Krizhevsky2009LearningML} dataset.
    }
    \label{tab:selected_models_ciphar}
    \setlength{\tabcolsep}{5pt}
    {\small
    \begin{tabular}{llcccccc}
    \toprule
    Dataset & Model & $L{-}1$ &  $d$ & Bound & Error$_{S}$ & Error$_{T}$ & MAP\\
    
    \end{tabular}
    }
\end{table}

\begin{table}[ht]
    \centering
    \caption{Extended details on the selected architecture in the experiments on wide architectures: number of hidden layers ($L{-}1$), width (d), both C and KL divergence values from the computation of the corresponding bound, learning rate (LR) and epoch providing the best model (Best epoch) given the algorithm stops after 100 epochs.
    }
    \label{tab:selected_models_details_mat_wide}
    \setlength{\tabcolsep}{5pt}
    {\small
    \begin{tabular}{llcccccc}
    \toprule
    Dataset & Model & $L{-}1$ &  $d$ & KL & C & LR & Best epoch\\
    \midrule
    \multirow{4}{*}{ads} 
    & PBGNet &  3 & 10 & 26 & 0.45 & 0.01 & 64 \\
    & ABNet &  2 & 10 & 29 & 0.47 & 0.01 & 51 \\
    & PBGNet$_{\ell}$ &  3 & 10 & 66262 & 17.33 & 0.001 & 55 \\
    & ABNet$_{\ell}$ &  2 & 50 & 20940 & 14.50 & 0.01 & 52 \\
    \midrule
    \multirow{4}{*}{adult} 
    & PBGNet &  1 & 10 & 238 & 0.30 & 0.1 & 87 \\
    & ABNet &  1 & 10 & 233 & 0.30 & 0.1 & 77 \\ 
    & PBGNet$_{\ell}$ &  2 & 10 & 3148 & 1.14 & 0.001 & 60  \\
    & ABNet$_{\ell}$ &  3 & 10 & 10014 & 1.93 & 0.01 & 52 \\
    \midrule
    \multirow{4}{*}{mnist17} 
    & PBGNet &  1 & 10 & 181 & 1.39 & 0.1 & 96 \\
    & ABNet &  1 & 10 & 171 & 1.35 & 0.1 & 78  \\
    & PBGNet$_{\ell}$ &  2 & 10 & 425542 & 17.33 & 0.1 & 19\\
    & ABNet$_{\ell}$ &  3 & 10 & 8578 & 6.66 & 0.01 & 33 \\
    \midrule
    \multirow{4}{*}{mnist49} 
    & PBGNet &  1 & 10 & 342 & 0.93 & 0.1 & 95  \\
    & ABNet &  1 & 10 & 329 & 0.91 & 0.1 & 86 \\
    &  PBGNet$_{\ell}$ &  1 & 50 & 39092 & 9.81 & 0.01 & 88\\
    & ABNet$_{\ell}$ &  3 & 10 & 158982 & 17.33 & 0.1 & 57  \\
    \midrule
    \multirow{4}{*}{mnist56} 
    & PBGNet &  1 & 10 & 202 & 0.95 & 0.01 & 87 \\
    & ABNet &  1 & 10 & 196 & 0.93 & 0.1 & 97 \\
    & PBGNet$_{\ell}$ &  1 & 50 & 35699 & 10.28 & 0.01 & 83  \\
    & ABNet$_{\ell}$ & 1 & 10 & 132207 & 17.33 & 0.1 & 82 \\
    \midrule
    \multirow{4}{*}{mnistLH} 
    & PBGNet &  1 & 10 & 1386 & 0.74 & 0.1 & 93 \\
    & ABNet & 2 & 10 & 1053 & 0.59 & 0.1 & 80 \\
    & PBGNet$_{\ell}$ &  1 & 100 & 262046 & 10.97 & 0.01 & 90 \\
    & ABNet$_{\ell}$ &  3 & 10 & 81752 & 5.02 & 0.01 & 68  \\
    \bottomrule
    \end{tabular}
    }
\end{table}

\begin{table}[ht]
    \centering
    \caption{Extended details on the extended experiments: number of hidden layers ($L{-}1$), width (d), both C and KL divergence values from the computation of the corresponding bound, learning rate (LR) and epoch providing the best model (Best epoch) given the algorithm stops after 100 epochs.
    }
    \label{tab:selected_models_ciphar_ext}
    \setlength{\tabcolsep}{5pt}
    {\small
    \begin{tabular}{llcccccc}
    \toprule
    Dataset & Model & $L{-}1$ &  $d$ & KL & C & LR & Best epoch\\
    \midrule
    \multirow{4}{*}{CIFAR10 - Truck VS Car} 
    & PBGNet & 1 & 10 & 177 & 0.42 & 0.1 & 118\\
    & ABNet & 1 & 10 & 172 & 0.41 & 0.01 & 70\\
    & PBGNet$_{\ell}$ & 1 & 50 & 39407 & 8.07 & 0.01 & 107\\
    & ABNet$_{\ell}$ & 2 & 50 & 5873 & 2.56 & 0.001 & 100\\
    \midrule
    \multirow{4}{*}{CIFAR10 - Cat VS Dog} 
    & PBGNet & 1 & 10 & 47 & 0.21 & 0.01 & 104\\
    & ABNet & 1 & 10 & 42 & 0.20 & 0.01 & 66\\
    & PBGNet$_{\ell}$ & 2 & 100 & 313085 & 17.33 & 0.001 & 57\\
    & ABNet$_{\ell}$ & 1 & 10 & 1699 & 1.30 & 0.001 & 71\\
    \midrule
    \multirow{4}{*}{CIFAR10 - Bird VS Plane} 
    & PBGNet & 1 & 10 & 92 & 0.29 & 0.01 & 87\\
    & ABNet & 1 & 10 & 86 & 0.28 & 0.01 & 81\\
    & PBGNet$_{\ell}$ & 1 & 100 & 65257 & 12.21 & 0.01 & 102\\
    & ABNet$_{\ell}$ & 3 & 10 & 3900 & 2.03 & 0.001 & 108\\
    \bottomrule
    \end{tabular}
    }
\end{table}
