# Supplementary material for: PAC-Bayesian Learning of Aggregated Binary Activated Neural Networks with Probabilities over Representations
Source: arXiv:2110.15137 source file (2023-04-14)
Supplement: Supplementary file 3 [file appendix_time.tex]

All experiments were performed on NVIDIA GPUs GeForce RTX 2080 Ti. We present an empirical study of computation time needed by our four algorithms (ABNet, Stochastic ABNet, Compact ABNet and Compact stochastic ABNet) and by the benchmark PBGNet (and its stochastic version) in Figures~\ref{fig:varying_width} and \ref{fig:varying_depth}. 

\begin{figure}[H]
  \centering
  \includegraphics[scale=0.85]{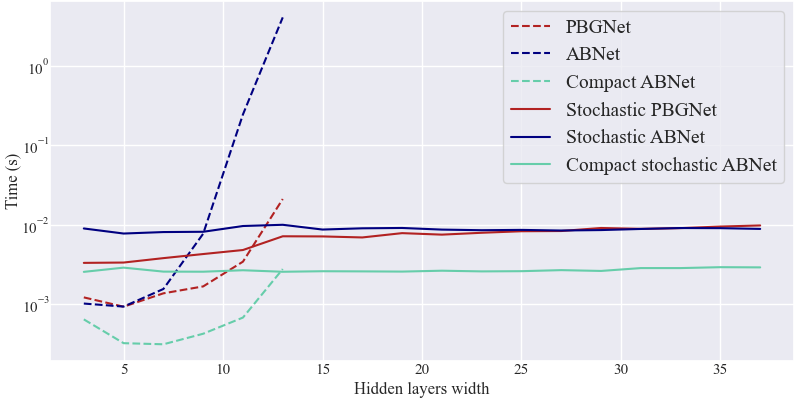}
  \caption{Time needed (in seconds) for the forward propagation of our four ABNet versions and the two versions of the PBGNet benchmark, all with $6$ hidden layers and with $100$ samples for stochastic versions. Computations were executed on a batch of 32 examples of the Ads dataset, averaged on 100 repetitions. Of note, the memory requirements of our (non-stochastic) PBGNet and ABNet
  implementations exceed the available resources for layer widths greater than 13. } 
  \label{fig:varying_width} 
\end{figure}

\begin{figure}[H]
  \centering
  \includegraphics[scale=0.85]{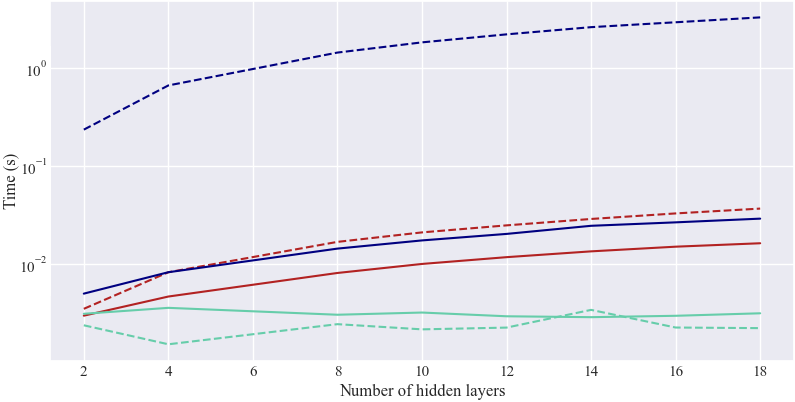}
  \caption{Time needed (in seconds) for the forward propagation of our four ABNet versions and the two versions of the PBGNet benchmark, all with width $d_k=12$ for $1 \leq k < L$, and with $100$ samples for stochastic versions. Computations were executed on a batch of 32 examples of the Ads dataset, averaged on 100 repetitions. See Figure~\ref{fig:varying_width} for the legend. }
  \label{fig:varying_depth} 
\end{figure}
